# Supplementary material for: LLMorpheus: Mutation Testing using Large Language Models
Source: arXiv:2404.09952 source file (2025-03-07)
Supplement: Supplementary file 4 [file table.tex]

\begin{table*}
 \centering
 {\scriptsize
 \begin{tabular}{l||r|r|r|r|r|r||r|r||r|r|r}
   {\bf application}                & {\bf \#prompts}   & {\bf \#mutants} & {\bf \#killed} & {\bf \#survived} & {\bf \#timeout} & \multicolumn{1}{|c||}{\bf mutation}   & \multicolumn{2}{|c||}{\bf time (sec)} & \multicolumn{3}{|c}{\bf \#tokens}\\
                                    &                   &                 &                &                  &                 & \multicolumn{1}{|c||}{\bf score}    & \ToolName & {\it StrykerJS}  & {\bf prompt} & {\bf completion} & {\bf total}\\
   \hline
   \textit{Complex.js} & 490 & 955 & 553 & 401 & 1 & 58.01 & 3,045.49 & 511.92 & 967,508 & 104,246 & 1,071,754 \\ 
   \hline
   \textit{countries-and-timezones} & 106 & 207 & 177 & 30 & 0 & 85.51 & 1,070.84 & 308.11 & 105,828 & 23,971 & 129,799 \\ 
   \hline
   \textit{crawler-url-parser} & 176 & 247 & 129 & 118 & 0 & 52.23 & 1,639.50 & 877.27 & 386,223 & 39,906 & 426,129 \\ 
   \hline
   \textit{delta} & 462 & 712 & 583 & 107 & 22 & 84.97 & 2,975.67 & 3,533.28 & 890,252 & 103,025 & 993,277 \\ 
   \hline
   \textit{image-downloader} & 42 & 77 & 48 & 29 & 0 & 62.34 & 430.50 & 458.40 & 24,655 & 9,339 & 33,994 \\ 
   \hline
   \textit{node-dirty} & 154 & 245 & 142 & 92 & 11 & 62.45 & 1,527.47 & 209.67 & 246,248 & 34,892 & 281,140 \\ 
   \hline
   \textit{node-geo-point} & 140 & 304 & 237 & 67 & 0 & 77.96 & 1,411.06 & 994.07 & 316,333 & 30,715 & 347,048 \\ 
   \hline
   \textit{node-jsonfile} & 68 & 137 & 43 & 45 & 49 & 67.15 & 690.64 & 421.39 & 57,516 & 15,398 & 72,914 \\ 
   \hline
   \textit{plural} & 153 & 208 & 154 & 53 & 1 & 74.52 & 1,521.06 & 112.22 & 265,602 & 34,926 & 300,528 \\ 
   \hline
   \textit{pull-stream} & 351 & 669 & 387 & 236 & 46 & 64.72 & 2,493.00 & 1,182.21 & 208,130 & 77,307 & 285,437 \\ 
   \hline
   \textit{q} & 1051 & 1715 & 122 & 1520 & 73 & 11.37 & 5,177.80 & 11,862.47 & 2,127,655 & 231,214 & 2,358,869 \\ 
   \hline
   \textit{spacl-core} & 134 & 185 & 160 & 25 & 0 & 86.49 & 1,350.98 & 606.49 & 162,705 & 30,694 & 193,399 \\ 
   \hline
   \textit{zip-a-folder} & 49 & 87 & 27 & 55 & 5 & 36.78 & 500.52 & 486.21 & 82,457 & 11,494 & 93,951 \\ 
   \hline
   \textit{Total} & 3376 & 5748 & 2762 & 2778 & 208 & - & 23,834.53  & 21,563.71 & 5,841,112 & 747,127 & 6,588,239 \\ 
 \end{tabular}
 }
 \caption{Results obtained with LLMorpheus using the following parameters: 
   model: \textit{codellama-13b-instruct}, 
   temperature: 0, 
   MaxTokens: 250, 
   MaxNrPrompts: 2000, 
   template: \textit{template-full.hb}, 
   systemPrompt: SystemPrompt-MutationTestingExpert.txt, 
   rateLimit: benchmark mode, 
   nrAttempts: 3  
 }
 \label{table:run358}
\end{table*}
